# Supplementary material for: Understanding and Improving the Efficiency of Full Configuration Interaction Quantum Monte Carlo
Source: arXiv:1601.00865 ancillary file (2016-03-14)
Supplement: Supplementary file 1 [file supp.pdf]

# Supplemental Material for "Understanding the Efficiency of Full Configuration Interaction Quantum Monte Carlo"

W. A. Vigor,[1] J. S. Spencer,[2,3] M. J. Bearpark,[1] and A. J. W. Thom[1,4]
[1)] Department of Chemistry, Imperial College London, Exhibition Road, London, SW7 2AZ, United Kingdom
[2)] Department of Physics, Imperial College London, Exhibition Road, London, SW7 2AZ, United Kingdom
[3)] Department of Materials, Imperial College London, Exhibition Road, London, SW7 2AZ, United Kingdom
[4)] University Chemical Laboratory, Lensfield Road, Cambridge, CB2 1EW, United Kingdom

(Dated: 15 February 2016)

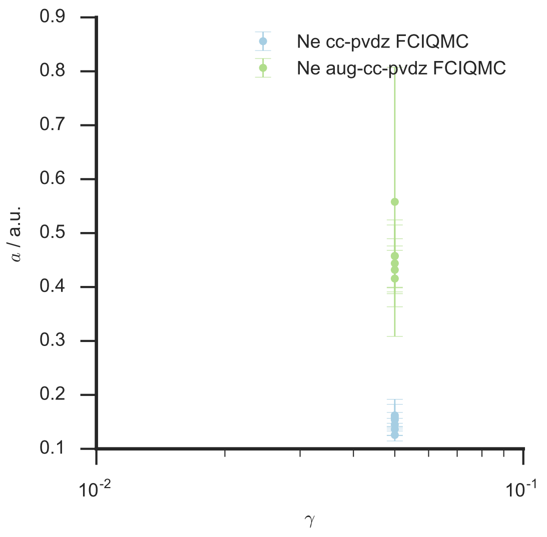


FIG. 1. The inefficiency $a$ as a function of $\gamma$. Using an estimate of the correlation energy we have adjusted $N_0$ and $\xi$ together to produce the same $\langle N_p \rangle$. For Ne cc-pVDZ we used $E_c \approx -0.19211$ $(\xi, N_0) =$ (0.1,146446), (0.5,680982), (0.75,774028), (1,825216), (1.25,857540), (1.5,879789) to give $\langle N_p \rangle = 1000000$. For Ne aug-cc-pVDZ we used $E_c \approx -0.21313$ $(\xi, N_0) =$ (0.1,118683), (0.5,652947), (0.75,752636), (1,808051), (1.25,843240), (1.5,867546) to give $\langle N_p \rangle = 1000000$. $\delta\tau$ was set to 0.005 for both Ne cc-pVDZ and Ne aug-cc-pVDZ.

Eq. 4 in the main text implies that $N_s$ and $\xi$ only have an impact on $\sigma_E$ by adjusting $\langle N_p \rangle$ and thus provide an extra degree of freedom. In Fig. 1 we show that this is the case even for systems with a significant sign problem such as Ne aug-cc-pVDZ, even though a choice of too large $\xi$ or too small a $\langle N_p \rangle$ will introduce a population control bias.[1] It is plausible that converging $\sigma_E$ to the same extent as in Ref. 1 would reveal an impact of population control on the inefficiency but in this case any such bias is masked by statistical error. We expect this behaviour to apply universally in FCIQMC.

We show the raw data for the behaviour of $a$ as function of $\langle N_p \rangle$ (Figs. 2 to 4) and hence find the value of

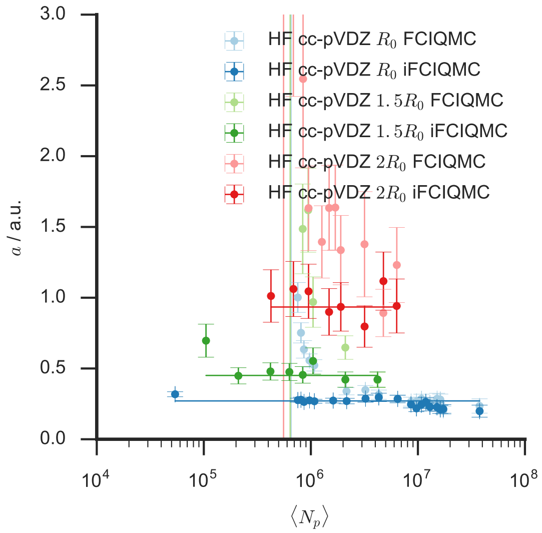


FIG. 2. The inefficiency $a$ for HF as a function of $\langle N_p \rangle$ and bond length ($R_0 = 0.91622$ Å). For $R = R_0$, $R = 1.5R_0$ and $R = 2R_0$ we used a $\delta\tau$ of 0.003, 0.001 and 0.001 respectively. These were determined using the data in Figs. 5 to 7.

$a_{\min}$ used in Sec. V of the main text. Further, the behaviour of $a$ with $\delta\tau$ is investigated for each system (Figs. 5 to 14) to demonstrate that the timestep used in Figs. 2 to 4 is smaller than $\delta\tau_0$. The additional purpose of this is to demonstrate that these observed behaviours are universal in FCIQMC/iFCIQMC for systems which have a significant plateau.

[1] W. A. Vigor, J. S. Spencer, M. J. Bearpark, and A. J. W. Thom, J. Chem. Phys. **142**, 104101 (2015).

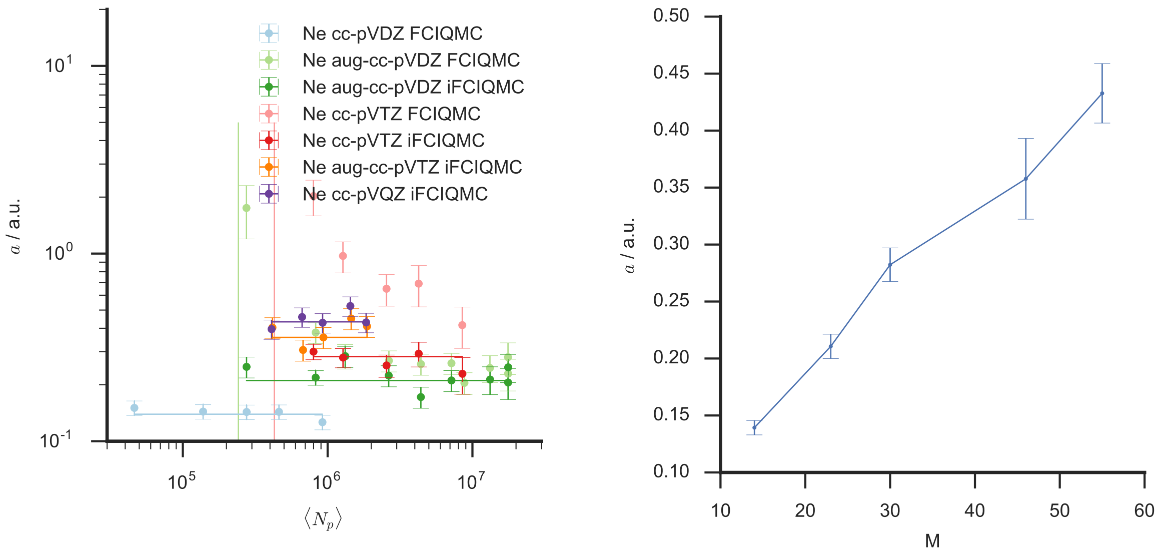


FIG. 3. Top: The inefficiency factor $a$ for the neon atom in a cc-pVDZ, aug-cc-pVDZ, cc-pVTZ, aug-cc-pVTZ and a cc-pVQZ basis set as a function of $\langle N_p \rangle$. Ne cc-pVDZ has no significant plateau and we find that $a$ is a constant function for $\langle N_p \rangle$. Bottom: the minimum value of $a$ as a function of basis set size. For Ne cc-pVDZ, Ne aug-cc-pVDZ, Ne cc-pVTZ, Ne aug-cc-pVTZ and Ne cc-pVQZ we used a $\delta\tau$ of 0.003606, 0.0022, 0.001075, 0.00065 and 0.00036 respectively (determined using the data in Fig. 2 (main text) and Fig. 8).

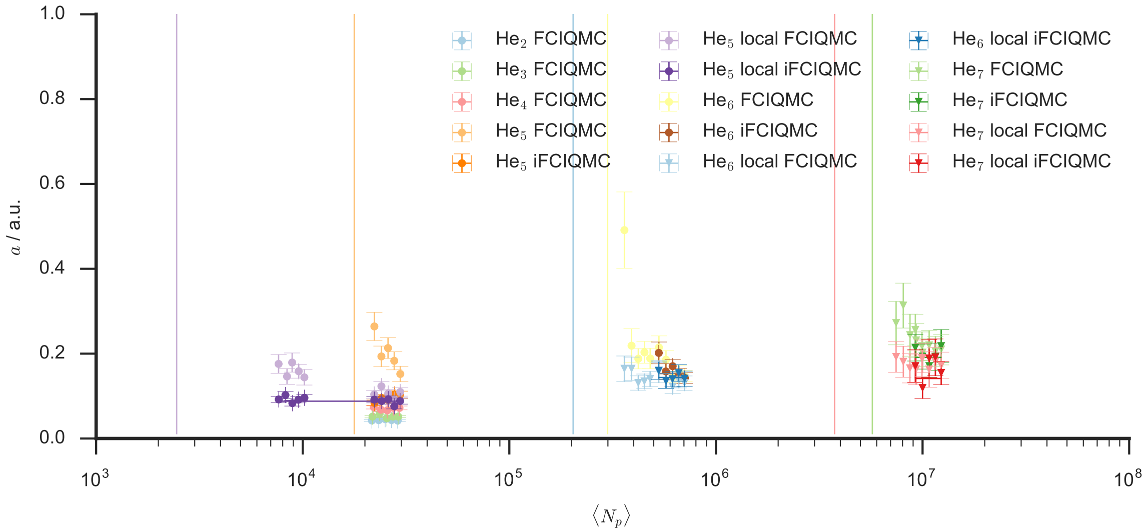


FIG. 4. The inefficiency $a$ as a function of $\langle N_p \rangle$ and number of atoms in a helium chain. A $\delta\tau$ of 0.02, 0.01, 0.005, 0.0042, 0.0036, 0.005, 0.0021 and 0.00175 was used for $He_3$, $He_4$, $He_5$, $He_6$, $He_7$ using canonical Hartree–Fock orbitals and $He_5$ $He_6$ and $He_7$ using localised orbitals respectively. The $\delta\tau$ used were determined in Figs. 9 to 14.

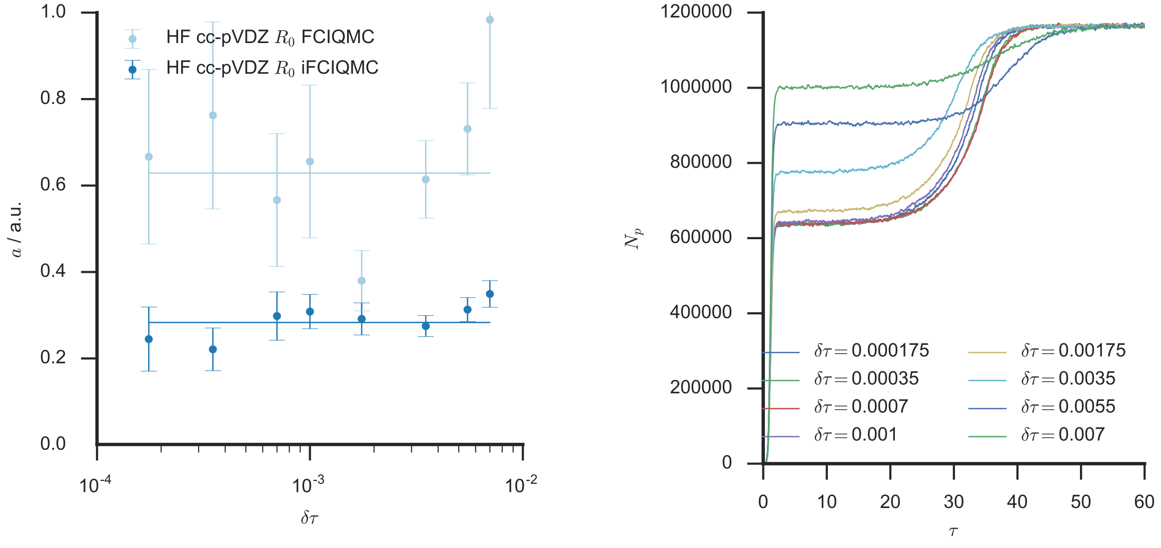


FIG. 5. Left: The inefficiency $a$ remains constant until $\delta\tau \approx 0.001$. Right: The plateau height can be seen to increase after $\delta\tau \approx 0.001$.

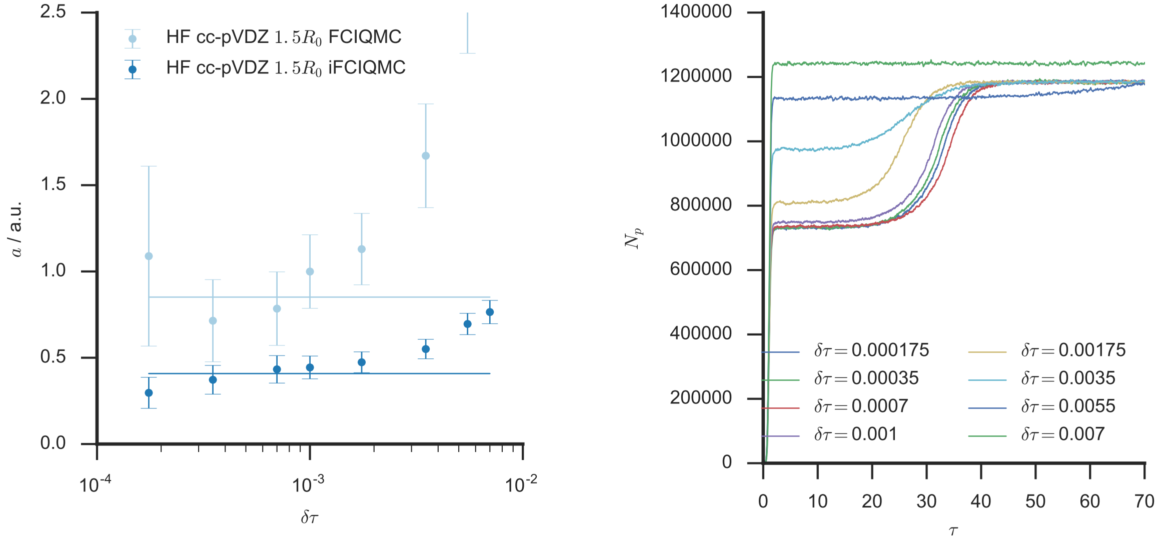


FIG. 6. Left: The inefficiency $a$ remains constant until $\delta\tau \approx 0.001$. Right: The plateau height can be seen to increase after $\delta\tau \approx 0.001$.

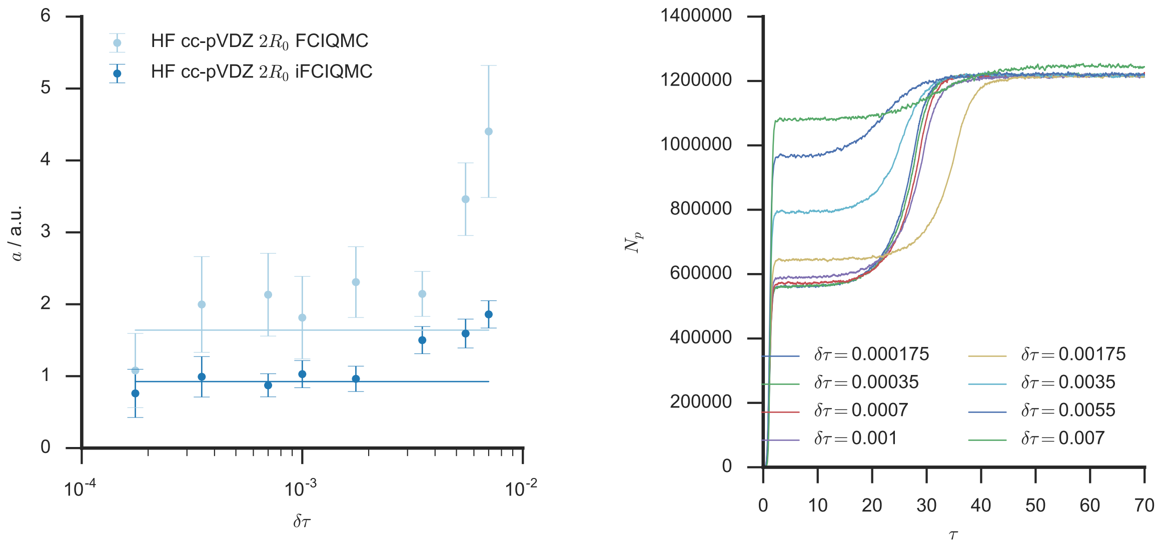


FIG. 7. Left: The inefficiency $a$ remains constant until $\delta\tau \approx 0.01$. Right: The plateau height can be seen to increase after $\delta\tau \approx 0.01$.

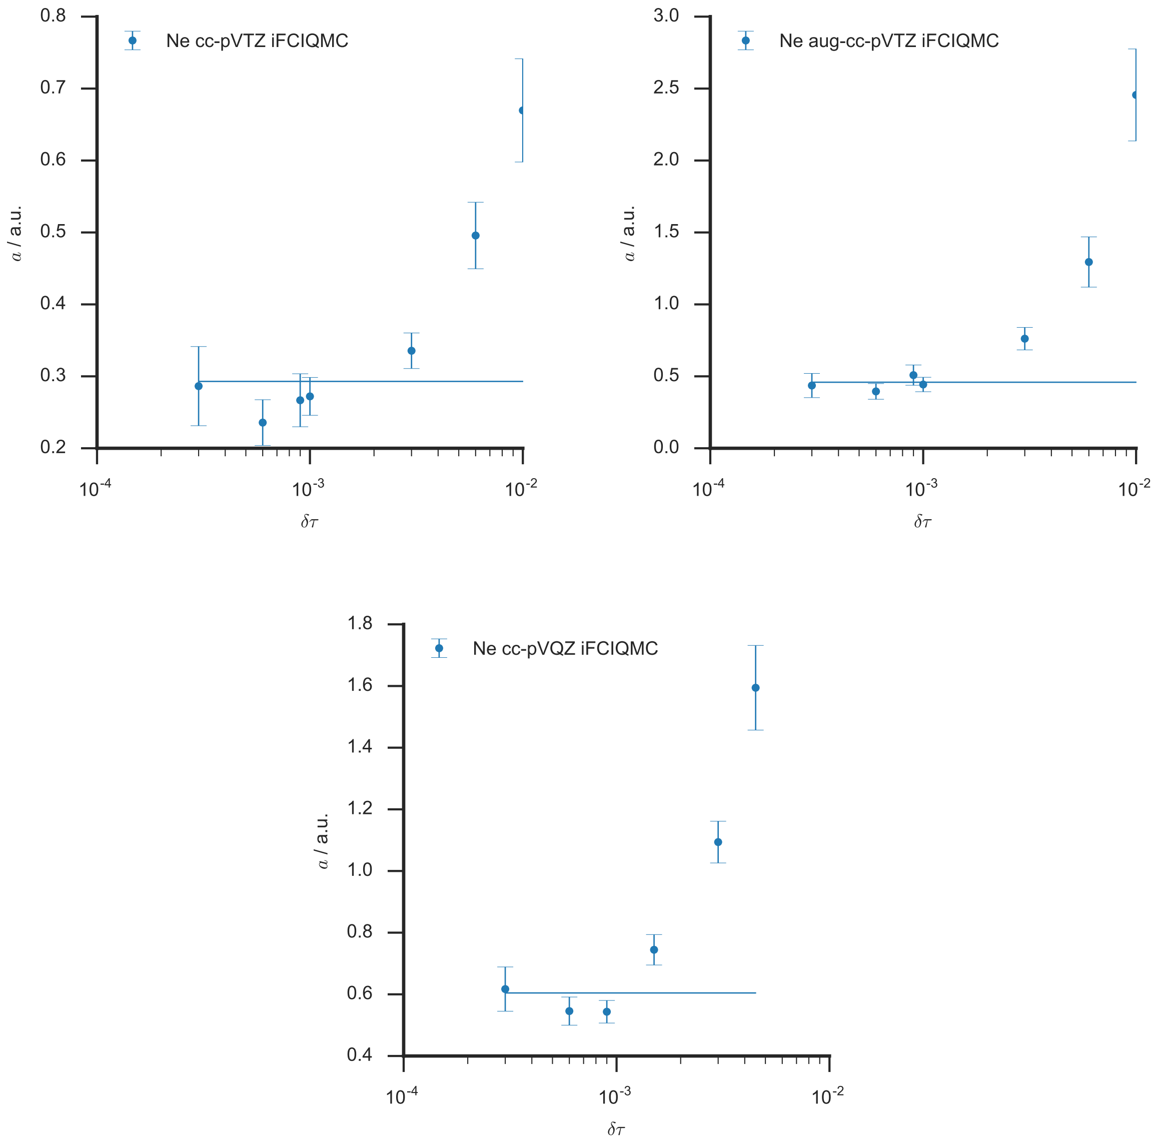


FIG. 8. Left: The inefficiency $a$ remains constant until $\delta\tau \approx 0.001$. Right: The inefficiency $a$ remains constant until $\delta\tau \approx 0.001$. Bottom: The inefficiency $a$ remains constant until $\delta\tau \approx 0.001$.

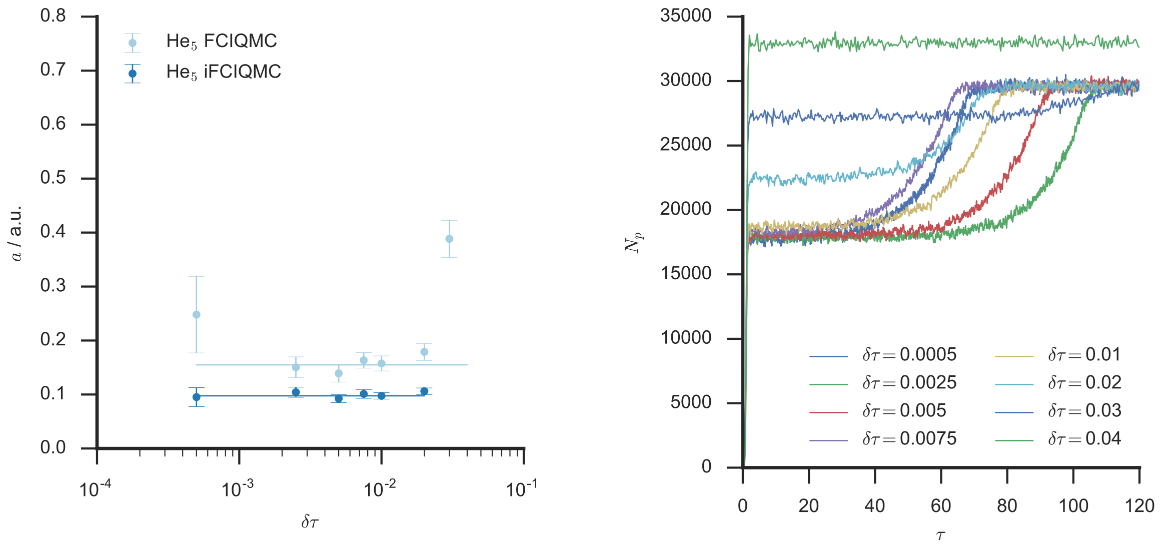


FIG. 9. Left: The inefficiency $a$ remains constant until $\delta\tau \approx 0.01$. Right: The plateau height can be seen to increase after $\delta\tau \approx 0.01$.

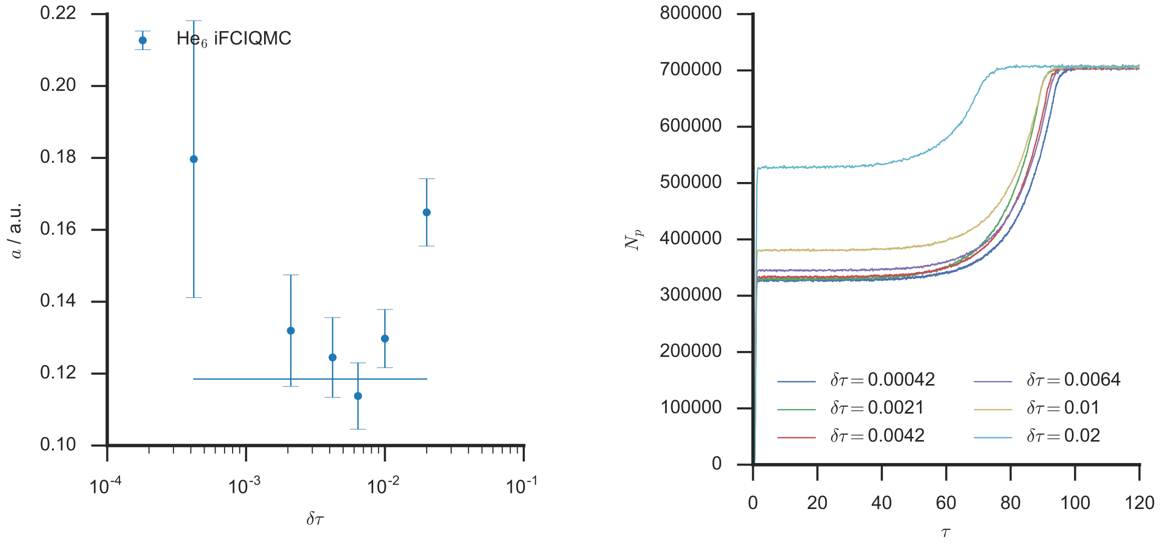


FIG. 10. Left: The inefficiency $a$ remains constant until $\delta\tau \approx 0.0042$. Right: The plateau height can be seen to increase after $\delta\tau \approx 0.0042$.

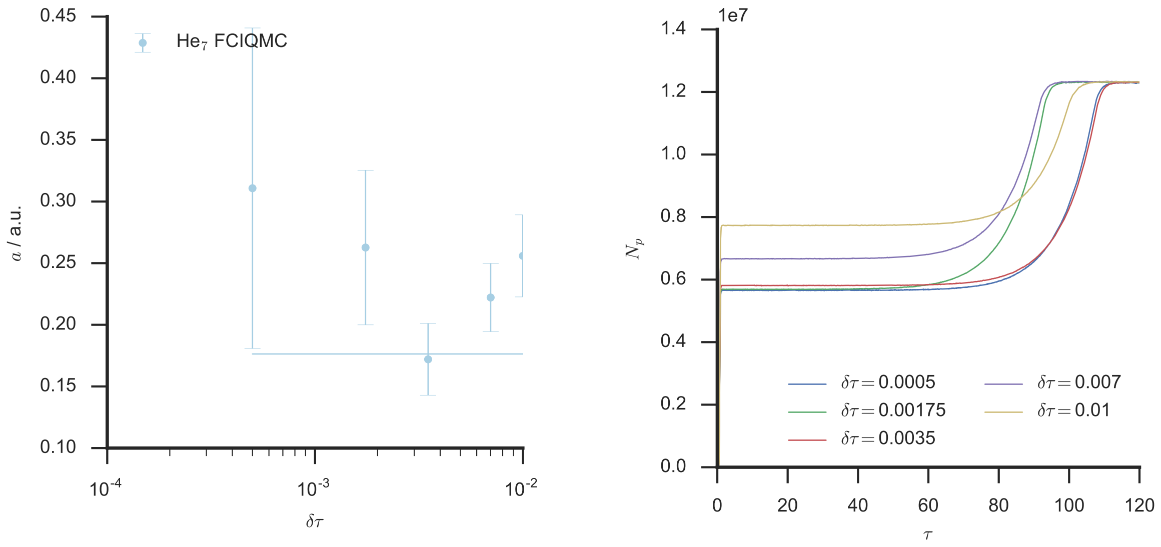


FIG. 11. Left: The inefficiency $a$ remains constant until $\delta\tau \approx 0.0035$. Right: The plateau height can be seen to increase after $\delta\tau \approx 0.0035$.

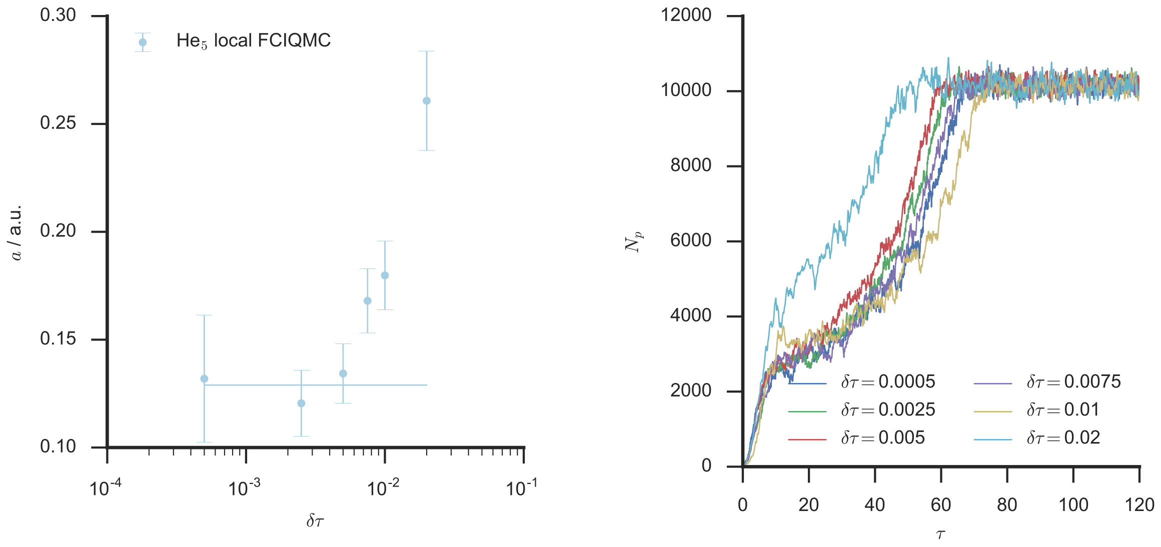


FIG. 12. Top: The inefficiency $a$ remains constant until $\delta\tau \approx 0.0005$. Bottom: The plateau height can be seen to increase after $\delta\tau \approx 0.0005$.

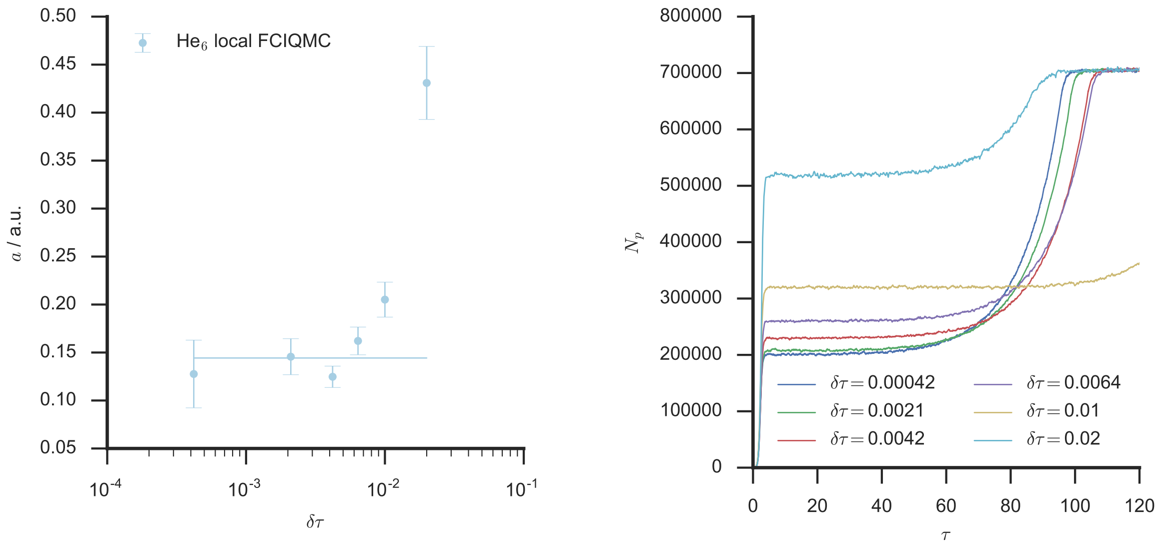


FIG. 13. Top: The inefficiency $a$ remains constant until $\delta\tau \approx 0.0021$. Bottom: The plateau height can be seen to increase after $\delta\tau \approx 0.0021$.

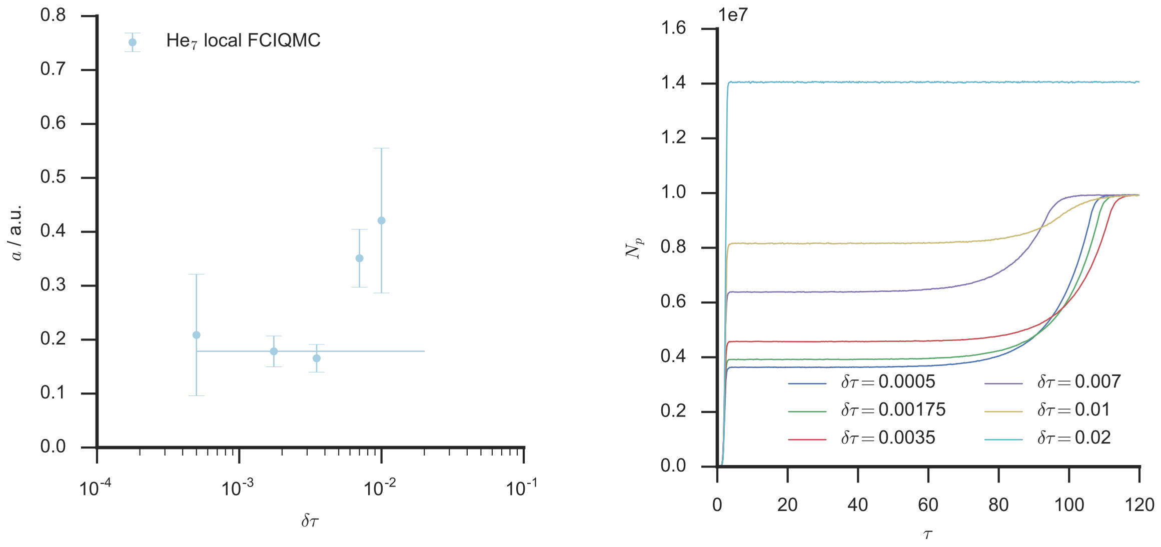


FIG. 14. Top: The inefficiency $a$ remains constant until $\delta\tau \approx 0.00175$. Bottom: The plateau height can be seen to increase after $\delta\tau \approx 0.00175$.
